# Supplementary material for: Outlier-Robust Clustering of Non-Spherical Mixtures
Source: arXiv:2005.02970 source file (2020-12-14)
Supplement: Supplementary file 1 [file appendix.tex]

\appendix

\section{Appendix}

\begin{Frame}[\textbf{Algorithm \ref{alg:row_norm_estimationn}} : Row Norm Estimation]
\label{alg:row_norm_estimationn}
\textbf{Input}: A PSD Matrix $\AA_{n \times n}$
\begin{enumerate}
    \item For $i \in [n]$, let $\mathcal{T}_i$ be a uniform random sample of $m = \Theta(k/\epsilon)$ indices in $[n]\setminus \{i\}$
    \item For $j \in [n]\setminus \{i\}$, let $\widetilde{Y}_j = \AA^2_{i,j}$ with probability $\frac{k}{\epsilon (n-1)}$ and $0$ otherwise. 
    \item Let $\widetilde{X}_i = \frac{(n-1)\epsilon}{k} \sum_{j \in  [n]\setminus \{i\}} \widetilde{Y}_j + \AA_{i,i}^2$
\end{enumerate}
\textbf{Output: Set $\{\widetilde{X}_1, \widetilde{X}_2, \ldots, \widetilde{X}_m \}$ }  
\end{Frame}

\begin{lemma}
Let $\AA$ be an $n \times n$ PSD matrix. For $i \in [n]$ let $\AA_{i, *}$ be the $i^{th}$ row of $\AA$. Algorithm $\ref{alg:row_norm_estimationn}$ uniformly samples $\Theta(k/\epsilon)$ indices from $[n]\setminus \{i\}$ along with diagonal index $i$ and  with probability at least $99/100$ outputs an estimator which obtains an $O(1)$-approximation to $\| \AA_{i, *} \|^2_2$. Further, the total running time of Algorithm $\ref{alg:row_norm_estimationn}$ is $O(\frac{kn}{\epsilon})$.
\end{lemma}

\begin{proof}
In step 1 of Algorithm \ref{alg:row_norm_estimationn} we sample $\Theta(k/\epsilon)$ entries in every row $i$ in PSD matrix $\AA$ along with its diagonal entries. Let  $\widetilde{X}_i = \frac{(n-1)\epsilon}{k} \sum_{j \in  [n]\setminus \{i\}} \widetilde{Y}_j + \AA_{i,i}^2$ where $\widetilde{Y}_{j}= \AA_{i,j}^2$ with probability  $\frac{k}{n\epsilon}$ and 0 otherwise. Then,

\begin{equation}
\begin{aligned}
\expecf{}{\widetilde{X}_i} & = \frac{n \epsilon}{k} \sum_{j \in [n] \setminus i} \expecf{}{Y_{i,j}} + \AA_{i,i}^2 \\
&= \frac{n \epsilon}{k} \sum_{j \in [n] \setminus i}  \frac{k}{n\epsilon} \AA_{i,j}^2 + \AA_{i,i}^2 \\
& = \| \AA_{i,*} \|^2_2   
\end{aligned}
\end{equation}
Using Chebyshev's Inequality we show that with high probability $\widetilde{X}_i$ is a constant factor approximation to $\| \AA_{i,*} \|^2_2$:

\begin{equation}
P\left[ \widetilde{X}_i  \geq (c+1) \| \AA_{i,*} \|^2_2 \right] \leq \frac{\varf{ \widetilde{X}_i}}{c^2 \| \AA_{i,*} \|^4_2}
\end{equation}
Where,

\begin{equation}
\begin{aligned}
\varf{ \widetilde{X}_i} = \varf{ \frac{n\epsilon}{k} \sum_{j \in [n]\setminus i} Y_{i,j} + \AA_{i,i}^2} &= \left( \frac{n\epsilon}{k} \right)^2 \varf{\sum_{j \in [n]\setminus i} Y_{i,j}} \\
& \leq \left( \frac{n\epsilon}{k} \right)^2 \EX((\sum_{j \in [n]\setminus i} Y_{i,j} )^2) \\
& = \left( \frac{n\epsilon}{k} \right)^2 \EX( \sum_{j \neq j'} Y_{i,j} Y_{i,j'} + \sum_{j \in [n]\setminus i} Y_{i,j}^2 ) \\
& = \left( \frac{n\epsilon}{k} \right)^2 \sum_{j \neq j'} \EX(Y_{i,j})  \EX(Y_{i,j'}) + \left( \frac{n\epsilon}{k} \right)^2 \sum_{j \in [n]\setminus i} \EX(Y_{i,j}^2) \\
& = \sum_{j \neq j'}  \AA_{i,j}^2  \AA_{i,j'}^2 +  \frac{n\epsilon}{k} \sum_{j \in [n]\setminus i}  \AA^4_{i, j} \\
& \leq \| \AA_{i,*} \|^4_2 + \frac{n\epsilon}{k} \sum_{j \in [n]\setminus i}  \AA^4_{i, j}
\end{aligned}
\end{equation}

Now our goal is to show that $\sum_{j \in [n]\setminus i}  \AA^4_{i, j} \leq \frac{k c'}{n\epsilon} \| \AA_{i,*} \|^4_2$ for some constant $c'$.
\end{proof}
